# Supplementary material for: Intrinsic conformal order revealed in geometrically confined long-range repulsive particles
Source: arXiv:2406.01053 source file (2024-06-03)
Supplement: Supplementary file 1 [file SI.pdf]

# Supplemental Material

Zhenwei Yao\*

*School of Physics and Astronomy, and Institute of Natural Sciences,*

*Shanghai Jiao Tong University, Shanghai 200240, China*

In this Supplemental Material, we provide more information about relevant theoretical derivations, details of numerical simulation, energy relaxation process and the effect of boundary stiffness, examples of conformal mapping, and the phenomenon of self-organization of dislocations in short-range interacting systems.

## I. THEORETICAL DERIVATIONS

### A. Derivation of the metric tensor

By mapping the point  $(x, y)$  in the  $z$ -plane to the point  $(u(x, y), v(x, y))$  in the  $\omega$ -plane, the distance  $ds_z$  of two points on the  $(x, y)$ -plane becomes  $ds_\omega$  on the  $(u, v)$ -plane.  $ds_z^2 = dx^2 + dy^2$ , and  $ds_\omega^2 = du^2 + dv^2$ . From

$$\begin{aligned} du &= \frac{\partial u}{\partial x} dx + \frac{\partial u}{\partial y} dy, \\ dv &= \frac{\partial v}{\partial x} dx + \frac{\partial v}{\partial y} dy. \end{aligned} \tag{1}$$

and the Cauchy–Riemann relation:

$$\begin{aligned} \frac{\partial u}{\partial x} &= \frac{\partial v}{\partial y}, \\ \frac{\partial u}{\partial y} &= -\frac{\partial v}{\partial x}. \end{aligned} \tag{2}$$

we have

$$du^2 + dv^2 = \left( \left( \frac{\partial u}{\partial x} \right)^2 + \left( \frac{\partial v}{\partial x} \right)^2 \right) (dx^2 + dy^2). \tag{3}$$

By inserting the following relation into Eq.(3)

$$\left| \frac{d\omega}{dz} \right|^2 = \frac{\partial(u, v)}{\partial(x, y)} = \left( \frac{\partial u}{\partial x} \right)^2 + \left( \frac{\partial v}{\partial x} \right)^2, \tag{4}$$

---

\*Electronic address: zyao@sjtu.edu.cn

we obtain

$$ds_\omega^2 = |\Lambda|^2 ds_z^2, \quad (5)$$

where  $|\Lambda| = |d\omega/dz|$ . We therefore have  $g_{xx} = g_{yy} = |\Lambda|^2$ , and  $g_{xy} = g_{yx} = 0$ . The intrinsic metric properties of the deformed triangular lattice is determined by the  $|\Lambda|$ -factor.

## B. Derivation of the Gaussian curvature

According to the Gauss's Theorema Egregium, the Gaussian curvature is an intrinsic property of the surface, and it is determined by the metric of the surface [1]. Specifically, for the surface parameterized by  $\vec{x}(u, v)$  with  $ds^2 = g_{uu}du^2 + g_{vv}dv^2$  ( $g_{uv} = g_{vu} = 0$ ), the Gaussian curvature is

$$K_G = -\frac{1}{\sqrt{g}} \left[ \partial_u \left( \frac{1}{\sqrt{g_{uu}}} \partial_u \sqrt{g_{vv}} \right) + \partial_v \left( \frac{1}{\sqrt{g_{vv}}} \partial_v \sqrt{g_{uu}} \right) \right]. \quad (6)$$

Over the 2D manifold with the following metric

$$ds_\omega^2 = |\Lambda|^2 ds_z^2, \quad (7)$$

we have  $g_{xx} = g_{yy} = |\Lambda|^2$ . By inserting the components of the metric tensor to Eq.(6), we obtain

$$K_G = \frac{1}{|\Lambda|^2} \Delta \ln \left( \frac{1}{|\Lambda|} \right) \quad (8)$$

## C. Derivation of the strain tensor

The conformal mapping from the point  $(x, y)$  in the  $z$ -plane to the point  $(u(x, y), v(x, y))$  in the  $\omega$ -plane could be regarded as a deformation of the original perfect triangular lattice with the displacement vector  $(X, Y)$ , where  $X = u - x$ , and  $Y = v - y$ . The line element over the deformed lattice can be written as

$$ds_\omega^2 = ds_z^2 + 2\epsilon_{\alpha\beta} dx_\alpha dx_\beta, \quad (9)$$

where  $x_1 = x$  and  $x_2 = y$ . The strain tensor is [2]

$$\epsilon_{\alpha\beta} = \frac{1}{2} \left( \frac{\partial u_\alpha}{\partial x_\beta} + \frac{\partial u_\beta}{\partial x_\alpha} + \frac{\partial u_\ell}{\partial x_\alpha} \frac{\partial u_\ell}{\partial x_\beta} \right), \quad (10)$$

where  $u_\alpha$  is the component of the displacement vector  $\vec{u}$  in the  $\hat{e}_\alpha$  direction. By inserting the displacement vector ( $u_x = X, u_y = Y$ ) into Eq.(10), we have

$$\begin{aligned}\epsilon_{xx} &= \frac{1}{2} \left[ \left( \frac{\partial u}{\partial x} \right)^2 + \left( \frac{\partial v}{\partial x} \right)^2 - 1 \right], \\ \epsilon_{yy} &= \frac{1}{2} \left[ \left( \frac{\partial u}{\partial y} \right)^2 + \left( \frac{\partial v}{\partial y} \right)^2 - 1 \right], \\ \epsilon_{xy} &= \epsilon_{yx} = 0.\end{aligned}\tag{11}$$

Due to the analyticity of the conformal transformation  $f(z)$ , the displacement field fulfills the Cauchy–Riemann relation [see Eq.(2)]. Note that there is a typo in the expression for  $\epsilon_{\alpha\beta}$  in Ref. [3]. Inserting the Cauchy–Riemann relation [Eq.(2)] into Eq.(11) leads to

$$\epsilon_{xx} = \epsilon_{yy},\tag{12}$$

We therefore reach the important conclusion that the conformal crystal could be obtained by locally isotropic deformation of a perfect triangular lattice.

## II. DETAILS OF NUMERICAL SIMULATION

We employ the steepest descent method to determine the equilibrium configuration of geometrically confined interacting particles. Given an initial configuration of particles, we first calculate the force on each particle. The force on the particle labelled  $i$  is denoted as  $\vec{F}_i$ , which includes both the interaction force from the other particles and that from the gradient of the confining potential (if the particle  $i$  is outside the box). The particle positions are then collectively updated by the force on them. Specifically, the particle  $i$  is moved by  $s_c \vec{f}_i$ , where  $s_c$  is the step size.  $\vec{f}_i = \vec{F}_i / F_{max}$ , where  $F_{max}$  is the maximum force on the particles. To fully eliminate the residue stress, we further update the particle positions individually at a finer step size until the total energy of the system reaches minimum. The typical step size for the collective and individual relaxation modes are  $s_c = 10^{-4} a_0$  and  $s_i = 0.1 s_c$ , respectively.  $a_0$  is the mean lattice spacing. In this force-driving protocol, each movement of the particles contributes to the reduction of the energy. Note that a full relaxation of the system at sufficiently fine step size is crucial for shaping defect-free zones. As has been pointed out in the main text, the energy difference between the intermediate configuration in Fig.1(a)

and the final equilibrium configuration in Fig.1(b) is very small. The combination of both collective and individual relaxation modes could efficiently eliminate the residue stress, and fully relax the system down to the energy valley.

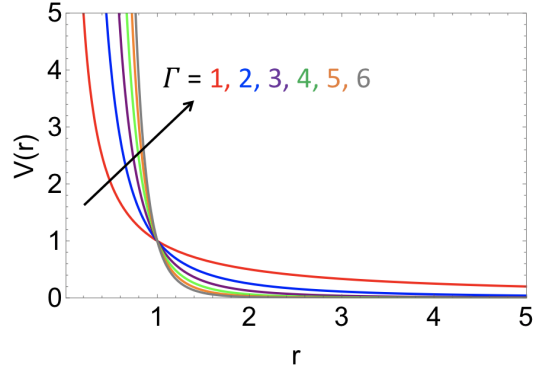

FIG. 1: Plot of the potential  $V(r)$  between interacting particles.  $V(r) = 1/r^\Gamma$ . The long-range feature of the Coulomb potential ( $\Gamma = 1$ ) is shown in the long tail of the curve.

In our numerical experiment, the particles interact by

$$V(r) = \frac{1}{r^\Gamma}, \quad (13)$$

where  $\Gamma$  is an integer. The potential curves  $V(r)$  for different values of  $\Gamma$  are plotted in Fig. 1. The long-range feature of the Coulomb potential ( $\Gamma = 1$ ) is shown in the long tail of the curve.

### III. MORE DATA ON ENERGY RELAXATION PROCESS AND THE EFFECT OF BOUNDARY STIFFNESS

Figure 2 shows the reduction of the total energy in the mechanical relaxation of the particle configuration. The relaxation process consists of collective and individual movements of the particles, as shown in Figs. 2(a) and 2(b). In the individual movements, a sweep consists of the movement of each particle by 1000 steps at the step size of  $10^{-4}a_0$ , where  $a_0$  is the mean lattice spacing. The typical particle configurations corresponding to the four sites on the energy curves are presented in the lower panels. It is observed that topological defects arise with the reduction of energy.

In Fig. 3, we show the persistence of the defect-free zone (highlighted by the light green hexagon) in the lowest-energy particle configurations at varying boundary stiffness. The

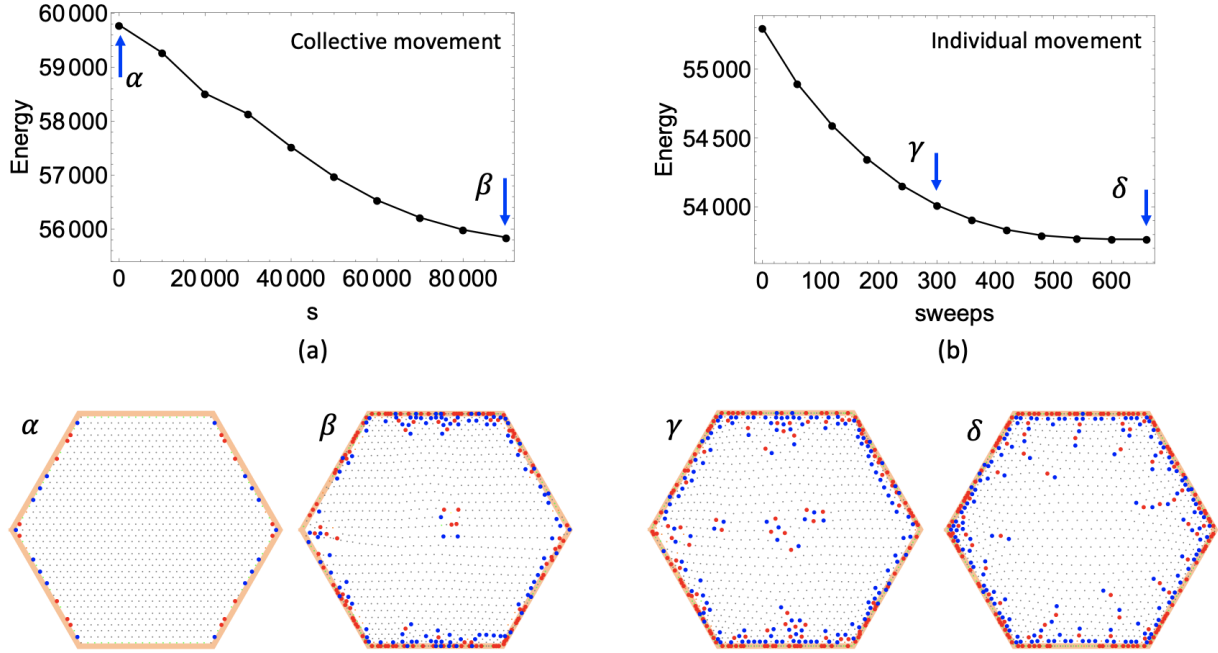

FIG. 2: Reduction of the total energy in the mechanical relaxation of the particle configuration. The typical particle configurations are presented in the lower panels. The outline in orange indicates the hexagonal boundary of the initial regular packing of particles in triangular lattice. The relaxation process consists of collective and individual movements of the particles. The red and blue dots in the interior of the disk represent five- and seven-fold disclinations.  $\Gamma = 1$ .  $N = 1141$ .

outline in orange indicates the hexagonal boundary of the initial regular packing of particles in triangular lattice. As the value of  $k_0$  is reduced to 10, Fig. 3(d) shows that the central region is still free of defects; a thin layer of particles are located outside the orange hexagonal outline.

#### IV. CONFORMAL MAPPING

The density profiles for both cases of  $\Gamma = 1$  and  $\Gamma = 2$  [see Fig.2(a) in the main text] can be realized by the conformal mapping defined as  $\omega = c'z^{1-\alpha/2}$  for  $\alpha \neq 2$ . In Fig. 4, the conformal transformations of the triangular lattice are visualized for different values of  $\alpha$ . We see the bending of the lattice and the appearance of inhomogeneity under the conformal transformation. The bond angle is preserved.

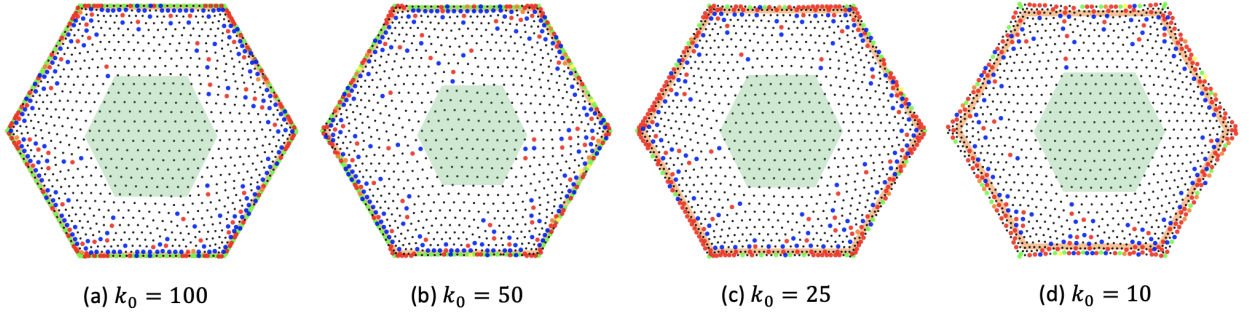

FIG. 3: Persistence of the defect-free zone in the lowest-energy particle configurations at varying boundary stiffness.  $k_0$  is the stiffness of the confining potential; see Eq.(2) in the main text. The defect-free zone is highlighted by the light green hexagon. The outline in orange indicates the hexagonal boundary of the initial regular packing of particles in triangular lattice.  $\Gamma = 1$ .  $N = 1141$ .

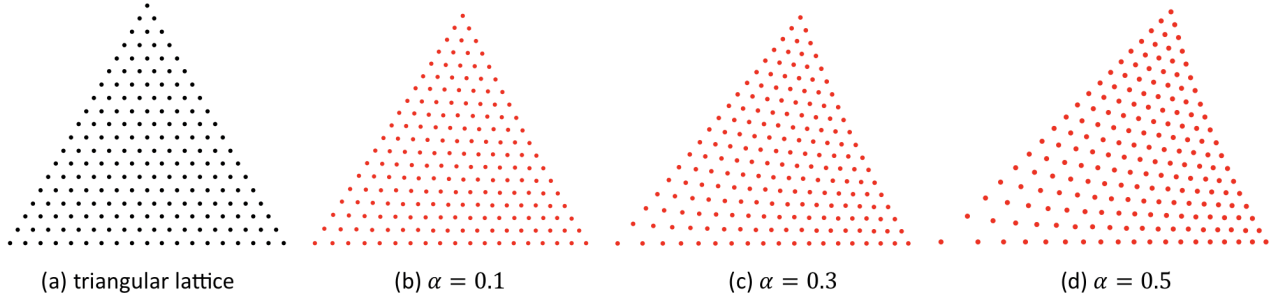

FIG. 4: Demonstration of the conformal transformations of the triangular lattice as defined by  $\omega(z) = c'z^{1-\alpha/2}$ .

## V. ORGANIZATION OF DISLOCATIONS INTO THE LOOP STRUCTURE

In this section, we provide more information about the spontaneous organization of dislocation into the loop structure in short-range interacting systems.

Simulations for the cases of  $\Gamma > 2$  show the appearance of multiple dislocations by changing the initial condition from the regular triangular lattice to the random configuration. More typical intermediate configurations in the relaxation process are presented in Fig. 5. The rightmost panel shows the equilibrium configuration. In the relaxation process, we see the formation of a long grain boundary across the entire system [see Fig. 5(a)-5(c)], and the aggregation of scattered dislocations to form the loop structure [see Fig. 5(d)-5(f)].

Here, we propose a heuristic argument for the formation of the loop structure composed of

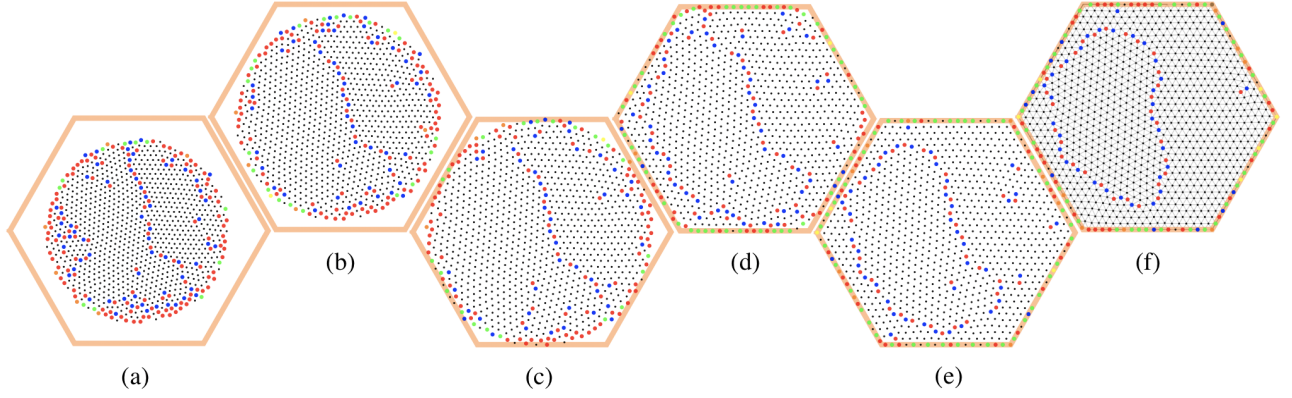

FIG. 5: Spontaneous aggregation of dislocations into the loop structure in the relaxation of the short-range interacting systems. The particles are initially randomly distributed in a circle [see (a)]. (a)-(f) Typical snapshots of the particle configuration in the relaxation process. The rightmost panel shows the equilibrium configurations. The red and blue dots in the interior of the disk represent five- and seven-fold disclinations.  $N = 1000$ .  $\Gamma = 6$ .

connecting dislocations. As the free-moving dislocations spontaneously aggregate to form the loop structure, the entropy associated with the configuration of the dislocations is reduced, indicating that this process is unfavored from the perspective of entropy. However, the head-tail connection of dislocations is energetically favored [4]. Therefore, the appearance of the loop structure could be qualitatively understood by the competition of the energy and the entropy. Once the loop structure is formed, the physical quantity of line tension emerges. Note that we observe the shrinking of the loop realized by the glide motions of dislocations. This process could be regarded as being driven by the line tension.

- 
- [1] D. Struik, *Lectures on Classical Differential Geometry* (Dover Publications, New York, 1988), 2nd ed.
  - [2] L. Landau and E. Lifshitz, *Theory of Elasticity* (Butterworth, Oxford, 1999).
  - [3] F. Rothen, P. Pieranski, N. Rivier, and A. Joyet, *Eur. J. Phys.* **14**, 227 (1993).
  - [4] P. Chaikin and T. Lubensky, *Principles of Condensed Matter Physics* (Cambridge University Press, 1995).
